# Supplementary material for: Accelerating Polynomial Multiplication for Homomorphic Encryption on GPUs
Source: arXiv:2209.01290 source file (2022-09-02)
Supplement: Supplementary file 1 [file 12_appendix.tex]

\section*{Appendix}

% Appendix is counted towards page count!

% __        __            _    ____                  _   
% \ \      / /__  _ __ __| |  / ___|___  _   _ _ __ | |_ 
%  \ \ /\ / / _ \| '__/ _` | | |   / _ \| | | | '_ \| __|
%   \ V  V / (_) | | | (_| | | |__| (_) | |_| | | | | |_ 
%    \_/\_/ \___/|_|  \__,_|  \____\___/ \__,_|_| |_|\__|

\begin{table}[ht]
	\centering % used for centering table
	\begin{tabular}{l c c} % centered columns (4 columns)
		\hline\hline %inserts double horizontal lines
		\textbf{Section} & \textbf{Word Count} & \textbf{Char Count} \\ [0.5ex] % inserts table
		%heading
		\hline % inserts single horizontal line
		Abstract & \quickwordcount{sections/01_abstract} & \quickcharcount{sections/01_abstract} \\
% 		Version 3 & 94.1\% \\ [1ex]
		\hline %inserts single line
	\end{tabular}
	\caption{Word counts for all sections} % title of Table
	\label{table:word_counts} % is used to refer this table in the text
\end{table}
